# Supplementary material for: Remote entanglement stabilization and distillation by quantum reservoir engineering
Source: arXiv:1703.03379 source file (2018-01-18)
Supplement: Supplementary file 1 [file remote_entanglement_stabilization_SM.pdf]

# Supplemental Material for "Remote entanglement stabilization and distillation by quantum reservoir engineering"

Nicolas Didier,[1,*] Jérémie Guillaud,[1] S. Shankar,[2] and Mazyar Mirrahimi[1,3]

[1] QUANTIC team, Inria Paris, 2 rue Simone Iff, 75012 Paris, France

[2] Departments of Applied Physics, Yale University, New Haven, Connecticut 06520, USA

[3] Yale Quantum Institute, Yale University, New Haven, Connecticut 06520, USA

## I. THREE-WAVE MIXER IN THE AMPLIFICATION MODE

### A. Low-rank approximation for simulating Lindblad equations

In this section, we recall the main ideas behind the low rank numerical method [S1] that we have used to simulate the remote entanglement protocol when the value of squeezing strength exceeds 8-10 dB. Indeed, when the squeezing exceeds 8 dB it is necessary to consider at least 10 Fock states in each cavity for numerical simulations, hence the density matrix is of size 400×400 or more. The low rank approximation method relies on the assumption that, even though the density matrix of the system $\rho$ might be large, only a small number of its eigenvectors are relevant, hence the effective rank of the matrix remains small (typically from 5 to 20). Replacing $\rho$ by a matrix of small rank thus produces a good approximation of the real density matrix.

In order to approximate the n×n density matrix $\rho$ by a matrix $\widetilde{\rho}$ of small rank m $\leq$ n, we decompose the latter in the following way

$$\widetilde{\rho} = U\sigma U^\dagger, \tag{S1}$$

where $\sigma$ is an m×m strictly positive Hermitian matrix, $U$ an n×m rectangular matrix such that $U^\dagger U = \mathbb{I}_m$,

A lifting procedure, described in details in [S1], yields the dynamics of $\sigma$ and $U$:

$$\frac{d}{dt}U = -iHU + (\mathbb{I}_n - UU^\dagger)\Big(\sum_\nu -\tfrac{1}{2}L_\nu^\dagger L_\nu + L_\nu U\sigma U^\dagger L_\nu^\dagger U\sigma^{-1}U^\dagger\Big)U \tag{S2}$$

$$\begin{aligned}\frac{d}{dt}\sigma = &\sum_\nu -\tfrac{1}{2}(U^\dagger L_\nu^\dagger L_\nu U\sigma + \sigma U^\dagger L_\nu^\dagger L_\nu U) + U^\dagger L_\nu U\sigma U^\dagger L_\nu^\dagger U \\ &+ \tfrac{1}{m}\mathrm{Tr}\Big(\sum_\nu L_\nu^\dagger(\mathbb{I}_n - UU^\dagger)L_\nu U\sigma U^\dagger\Big)\mathbb{I}_m\end{aligned} \tag{S3}$$

The approximate matrix $\widetilde{\rho}$ is thus computed as follows: given the initial state $\rho_0$, we compute initial matrix $U_0$ and $\sigma_0$ so that $\widetilde{\rho}_0 = U_0\sigma_0 U_0^\dagger$ is a good approximation of $\rho_0$. The above dynamics are then numerically integrated, and we finally form the product $\widetilde{\rho} = U\sigma U^\dagger$ to obtain the low rank approximation of the real density matrix $\rho$.

Here, we provide the steps of the numerical algorithm, to integrate the above dynamics:

*a. Initial condition* In all the simulations presented below, the inital state is $|\psi_0\rangle = |00\rangle \otimes |gg\rangle$, i.e both qubits are in the ground state and cavities are empty. The corresponding initial density matrix is $\rho_0 = |\psi_0\rangle\langle\psi_0|$, of rank 1. For this particular $\rho_0$, $\sigma_0$ is a diagonal matrix where the first element is $1-(m-1)\epsilon$ and the other ones are $\epsilon$, where $\epsilon \ll 1$ ($\epsilon = 10^{-10}$ in our simulations), and $U_0$ is given by $U_0 = \Upsilon\big([|\psi_0\rangle, S|\psi_0\rangle, ..., S^{m-1}|\psi_0\rangle]\big)$, where $S = H - \sum_\nu \frac{1}{2}L_\nu^\dagger L_\nu$ and $\Upsilon$ denotes a Gram-Schmidt orthonormalization procedure.

*b. Integration of the dynamics* The discretization of the above dynamics for $U$ and $\sigma$ needs to be done carefully, so as to ensure that the density matrix $\rho$ remains positive and of trace 1 at all times. We use the Trotter scheme of [S1]. It is divided in three steps :

* Current address: Rigetti Computing, 775 Heinz Avenue, Berkeley, California 94710, USA.

1. Free Hamiltonian evolution over a time $\delta t/2$, $U_{k+\frac{1}{3}} = e^{-i\delta t/2H}U_k$ thanks to the third order expansion:

$$U_{k+\frac{1}{3}} = \Big(\mathbb{I}_n - i\frac{\delta t}{2}H - \frac{\delta t^2}{8}H + i\frac{\delta t^3}{48}H\Big)U_k \tag{S4}$$

2. Updating $U$ and $\sigma$ accounting for the dissipation process :

$$U_{k+\frac{2}{3}} = U_{k+\frac{1}{3}} + \delta t(\mathbb{I}_n - U_{k+\frac{1}{3}}U^\dagger_{k+\frac{1}{3}})\Big(\sum_\nu -\tfrac{1}{2}L^\dagger_\nu L_\nu U_{k+\frac{1}{3}} + L_\nu U_{k+\frac{1}{3}}\sigma_k U^\dagger_{k+\frac{1}{3}}L^\dagger_\nu U_{k+\frac{1}{3}}\sigma_k^{-1}\Big),$$

$$\begin{aligned}\sigma_{k+\frac{1}{2}} = \sigma_k + \delta t\sum_\nu \Big[&U^\dagger_{k+\frac{1}{3}}L_\nu U_{k+\frac{1}{3}}\sigma_k U^\dagger_{k+\frac{1}{3}}L^\dagger_\nu U_{k+\frac{1}{3}} \\ &+ \frac{\delta t}{m}\mathrm{Tr}\Big((U^\dagger_{k+\frac{1}{3}}L^\dagger_\nu L_\nu U_{k+\frac{1}{3}} - U^\dagger_{k+\frac{1}{3}}L^\dagger_\nu U_{k+\frac{1}{3}}U^\dagger_{k+\frac{1}{3}}L_\nu U_{k+\frac{1}{3}})\sigma_k\Big)\mathbb{I}_m\Big],\end{aligned} \tag{S5}$$

$$\sigma_{k+1} = \frac{(\mathbb{I}_m - \frac{\delta t}{2}\sum_\nu U^\dagger_{k+\frac{1}{3}}L^\dagger_\nu L_\nu U_{k+\frac{1}{3}})\sigma_{k+\frac{1}{2}}(\mathbb{I}_m - \frac{\delta t}{2}\sum_\nu U^\dagger_{k+\frac{1}{3}}L^\dagger_\nu L_\nu U_{k+\frac{1}{3}})}{\mathrm{Tr}\Big((\mathbb{I}_m - \frac{\delta t}{2}\sum_\nu U^\dagger_{k+\frac{1}{3}}L^\dagger_\nu L_\nu U_{k+\frac{1}{3}})\sigma_{k+\frac{1}{2}}(\mathbb{I}_m - \frac{\delta t}{2}\sum_\nu U^\dagger_{k+\frac{1}{3}}L^\dagger_\nu L_\nu U_{k+\frac{1}{3}})\Big)},$$

3. Once again a free Hamiltonian evolution over a time $\delta t/2$, this time followed by an orthonormalization (denoted $\Upsilon$) to ensure $U^\dagger_{k+1}U_{k+1} = \mathbb{I}_m$:

$$U_{k+1} = \Upsilon\Big(\Big(\mathbb{I}_n - i\frac{\delta t}{2}H - \frac{\delta t^2}{8}H + i\frac{\delta t^3}{48}H\Big)U_{k+\frac{2}{3}}\Big), \tag{S6}$$

The dynamics simulated in this paper corresponds to the Lindblad master equation where the hamiltonian and the Lindblad operators are given by

$$\begin{aligned}&\hat{H} = \hat{H}_{\text{dispersive}} + \hat{H}_{\text{drive}} = -\tfrac{1}{2}\hbar\chi(\hat{a}_1^\dagger\hat{a}_1\hat{\sigma}_{z,1} + \hat{a}_2^\dagger\hat{a}_2\hat{\sigma}_{z,2}) + \tfrac{1}{2}\hbar\Omega(\hat{\sigma}_{x,1} + \hat{\sigma}_{x,2}) \\ &\hat{L}_1 = \sqrt{\eta\kappa}(\hat{a}_1\,\cosh(\mathrm{r}) + \hat{a}_2^\dagger\,\sinh(\mathrm{r})), \quad \hat{L}_2 = \sqrt{\eta\kappa}(\hat{a}_2\,\cosh(\mathrm{r}) + \hat{a}_1^\dagger\,\sinh(\mathrm{r})) \\ &\hat{L}_3 = \sqrt{(1-\eta)\kappa}\;\hat{a}_1, \quad \hat{L}_4 = \sqrt{(1-\eta)\kappa}\;\hat{a}_2.\end{aligned} \tag{S7}$$

For an efficiency $\eta < 1$, the operators $\hat{L}_3$, $\hat{L}_4$ take into account the finite efficiency of the transmissions lines.

For a simulation with the following parameters: $r_{dB} = 10$ dB, $N_{ph} = 12$, $\kappa/2\pi = 1$MHz, $\chi = 5\kappa$, $\Omega = 1.6\kappa$, $\eta = 1$, $T_{sim} = 40/\kappa$ an integration on QuTiP takes 16 minutes and 11 seconds, while the low rank algorithm (with low rank $m = 5$) takes 1 minute 48 seconds (Processor: Intel(R) Core(TM) i7-6500U CPU @2.50GHz).

## B. Convergence analysis in the amplification mode

### 1. *Stabilization scheme detailed mecanism*

As explained in the main text, the entanglement stabilization in the amplification mode can be understood in the following way: in the absence of the qubit drives, the cavities admit a joint pointer state that depends on the parity of the qubits. When the qubits are in an odd state span$\{|ge\rangle, |eg\rangle\}$, the cavities pointer state is the squeezed vacuum state, and when the qubits are in an even state span$\{|gg\rangle, |ee\rangle\}$, the cavities pointer state is a squeezed thermal state. In this section, we provide a proof for this claim.

We recall that each qubit is dispersively coupled to its own cavity, an interaction governed by the following Hamiltonian : $\hat{H}_{\text{dispersive},j=1,2} = -\frac{1}{2}\hbar\chi_j\hat{a}_j^\dagger\hat{a}_j\hat{\sigma}_{z,j}$. When the qubit/cavity coupling is identical in both cavities ($\chi_1 = \chi_2 = \chi$), it is useful to decompose this Hamiltonian on the odd and even qubits subspaces:

$$\hat{H}_{\text{dispersive}} = \frac{\hbar\chi}{2}\hat{N}(\hat{\sigma}_{\text{gg}} - \hat{\sigma}_{\text{ee}}) + \frac{\hbar\chi}{2}\hat{M}(\hat{\sigma}_{eg} - \hat{\sigma}_{ge}), \tag{S8}$$

where

$$\hat{\sigma}_{\rm gg} = |{\rm gg}\rangle\langle{\rm gg}|, \quad \hat{\sigma}_{\rm ee} = |{\rm ee}\rangle\langle{\rm ee}|, \quad \hat{\sigma}_{\rm ge} = |{\rm ge}\rangle\langle{\rm ge}|, \quad \hat{\sigma}_{\rm eg} = |{\rm eg}\rangle\langle{\rm eg}|,$$
$$\hat{N} = \hat{a}_1^\dagger\hat{a}_1 + \hat{a}_2^\dagger\hat{a}_2, \quad \hat{M} = \hat{a}_1^\dagger\hat{a}_1 - \hat{a}_2^\dagger\hat{a}_2, \tag{S9}$$

$\hat{N}$ and $\hat{M}$ being the photon number sum and difference, respectively.

*a. Qubits in odd manifold* Suppose that the qubits are in the odd qubit subspace. The interaction Hamiltonian reduces to :

$$\hat{H}_{\rm dispersive} = \frac{\hbar\chi}{2}\hat{M}(\hat{\sigma}_{eg} - \hat{\sigma}_{ge}). \tag{S10}$$

We now perform the following Bogoliubov transformation

$$\hat{b}_1 = \hat{a}_1 \cosh({\rm r}) + \hat{a}_2^\dagger \sinh({\rm r}), \quad \hat{b}_2 = \hat{a}_2 \cosh({\rm r}) + \hat{a}_1^\dagger \sinh({\rm r}). \tag{S11}$$

Note that the photon number difference operator $\hat{M}$ is left invariant by this transformation

$$\hat{M}_{\hat{b}} = \hat{b}_1^\dagger\hat{b}_1 - \hat{b}_2^\dagger\hat{b}_2 = \hat{a}_1^\dagger\hat{a}_1 - \hat{a}_2^\dagger\hat{a}_2 = \hat{M}. \tag{S12}$$

The dynamics thus reads

$$\frac{d\rho}{dt} = -i[\hat{H}_{\rm disp}, \rho] + \sum_{\nu=1,2} \hat{L}_\nu\rho\hat{L}_\nu^\dagger - \tfrac{1}{2}(\hat{L}_\nu^\dagger\hat{L}_\nu\rho + \rho\hat{L}_\nu^\dagger\hat{L}_\nu) \tag{S13}$$

with $\hat{H}_{\rm disp} = \frac{\hbar\chi}{2}\hat{M}_{\hat{b}}(\hat{\sigma}_{eg} - \hat{\sigma}_{ge})$, $\hat{L}_1 = \sqrt{\kappa}\hat{b}_1$, and $\hat{L}_2 = \sqrt{\kappa}\hat{b}_2$.

It is clear that the steady state of this dynamics is $\bar{\rho} = |00\rangle\langle 00| \otimes \rho_q$ where $|00\rangle$ is the vacuum state of the Bogoliubov modes $\hat{b}_1$ and $\hat{b}_2$ and $\rho_q$ is the qubits state in the odd manifold. It is known that the Bogoliubov vacuum correspond to the two-mode squeezed state in the original basis $\hat{a}_1$, $\hat{a}_2$.

*b. Qubits in even manifold* Suppose now that the qubits are in the even qubits subspace. The interaction Hamiltonian reduces to

$$\hat{H}_{\rm dispersive} = \frac{\hbar\chi}{2}\hat{N}(\hat{\sigma}_{gg} - \hat{\sigma}_{ee}). \tag{S14}$$

We consider the case where both qubits are in the ground state, i.e the density matrix of the whole system is given by $\rho = \rho_c \otimes |gg\rangle\langle gg|$ (the case where both qubits are in the excited state can be treated in the same manner). The dynamics of the reduced density matrix of the cavities is then given by

$$\frac{d\rho_c}{dt} = -i[\hat{H}_{\rm disp}, \rho_c] + \sum_{\nu=1,2} \hat{L}_\nu\rho_c\hat{L}_\nu^\dagger - \tfrac{1}{2}(\hat{L}_\nu^\dagger\hat{L}_\nu\rho_c + \rho_c\hat{L}_\nu^\dagger\hat{L}_\nu) \tag{S15}$$

with $\hat{H}_{\rm disp} = \pm\frac{\hbar\chi}{2}\hat{N}$ ($+$ for $|gg\rangle$ and $-$ for $|ee\rangle$), $\hat{L}_1 = \sqrt{\kappa}(\hat{a}_1 \cosh({\rm r}) + \hat{a}_2^\dagger \sinh({\rm r}))$, and $\hat{L}_2 = \sqrt{\kappa}(\hat{a}_2 \cosh({\rm r}) + \hat{a}_1^\dagger \sinh({\rm r}))$. To compute the steady state of this dynamics, we use the characteristic functions formalism [S2, S3]. For a two-mode field, the characteristic function is given by:

$$\Phi(t, \xi, \eta) = {\rm Tr}[\rho(t)\, \exp(\xi\hat{a}_1^\dagger - \xi^*\hat{a}_1)\exp(\eta\hat{a}_2^\dagger - \eta^*\hat{a}_2)]. \tag{S16}$$

The dynamics for $\rho_c$ can be transformed into a partial differential equation for the characteristic function. Solving the equation yields the steady state as well as the rate of convergence to the solution. Using the rules of correspondance given in [S2], we get the following dynamics for $\Phi$ :

$$\begin{aligned}\frac{1}{\kappa}\frac{\partial\Phi}{\partial t} =& \mp \frac{\chi}{2\kappa}(\xi^*\frac{\partial}{\partial\xi^*} - \xi\frac{\partial}{\partial\xi} + \eta^*\frac{\partial}{\partial\eta^*} - \eta\frac{\partial}{\partial\eta})\Phi - \frac{1}{2}(x.\nabla)\Phi \\ &- \frac{1}{2}[(|\eta|^2 + |\xi|^2){\rm cosh}(2{\rm r}) + (\xi\eta + \xi^*\eta^*){\rm sinh}(2{\rm r})]\Phi,\end{aligned} \tag{S17}$$

where

$$x.\nabla = \xi^* \frac{\partial}{\partial \xi^*} + \xi \frac{\partial}{\partial \xi} + \eta^* \frac{\partial}{\partial \eta^*} + \eta \frac{\partial}{\partial \eta}.$$

We solve this equation using the method of the characteristics. Writing $\xi = x_1 + iy_1$ and $\eta = x_2 + iy_2$, where $x_i$, $y_i$, $i = 1, 2$ are real variables, the equation becomes :

$$\begin{aligned} \frac{1}{\kappa}\frac{\partial \Phi}{\partial t} = & -\frac{1}{2}\big((x_1 \pm \frac{\chi}{\kappa} y_1)\frac{\partial}{\partial x_1} + (x_2 \pm \frac{\chi}{\kappa} y_2)\frac{\partial}{\partial x_2} + (y_1 \mp \frac{\chi}{\kappa} x_1)\frac{\partial}{\partial y_1} + (y_2 \mp \frac{\chi}{\kappa} x_2)\frac{\partial}{\partial y_2}\big)\Phi \\ & -\frac{1}{2}[(x_1^2 + y_1^2 + x_2^2 + y_2^2)\cosh(2\mathrm{r}) + 2(x_1 x_2 - y_1 y_2)\sinh(2\mathrm{r})]\Phi. \end{aligned} \tag{S18}$$

On the characteristic curves, we have:

$$\begin{aligned} \kappa dt &= \frac{2dx_1}{x_1 \pm \frac{\chi}{\kappa} y_1} = \frac{2dx_2}{x_2 \pm \frac{\chi}{\kappa} y_2} = \frac{2dy_1}{y_1 \mp \frac{\chi}{\kappa} x_1} = \frac{2dy_2}{y_2 \mp \frac{\chi}{\kappa} x_2} \\ &= \frac{-2d\Phi}{[(x_1^2 + y_1^2 + x_2^2 + y_2^2)\cosh(2\mathrm{r}) + 2(x_1 x_2 - y_1 y_2)\sinh(2\mathrm{r})]\Phi}. \end{aligned} \tag{S19}$$

Integrating the first line of the above equations, we get the following expressions on a characteristic

$$\begin{pmatrix} x_1 \\ y_1 \end{pmatrix} = e^{\frac{\kappa t}{2}} \begin{pmatrix} \cos\frac{\chi t}{2} & \pm\sin\frac{\chi t}{2} \\ \mp\sin\frac{\chi t}{2} & \cos\frac{\chi t}{2} \end{pmatrix} \begin{pmatrix} K_1 \\ K_2 \end{pmatrix}, \quad \begin{pmatrix} x_2 \\ y_2 \end{pmatrix} = e^{\frac{\kappa t}{2}} \begin{pmatrix} \cos\frac{\chi t}{2} & \pm\sin\frac{\chi t}{2} \\ \mp\sin\frac{\chi t}{2} & \cos\frac{\chi t}{2} \end{pmatrix} \begin{pmatrix} K_3 \\ K_4 \end{pmatrix}. \tag{S20}$$

Here $K_i$'s are real constants and their choice determines the characteristic. Plugging these expressions into the last equation, we get

$$\big[C_1 + 2[C_2 \cos\chi t \pm C_3 \sin\chi t]\big]\kappa e^{\kappa t} dt = -2\frac{d\Phi}{\Phi}, \tag{S21}$$

where $C_1 = (K_1^2 + K_2^2 + K_3^2 + K_4^2)\cosh(2\mathrm{r})$, $C_2 = (K_1 K_3 - K_2 K_4)\sinh(2\mathrm{r})$, $C_3 = (K_1 K_4 + K_2 K_3)\sinh(2\mathrm{r})$. Integrating this equation, we get

$$\begin{aligned} \Phi(t, \xi, \eta) = C_4 \ \exp\Big\{ -\frac{1}{2}\big[C_1 e^{\kappa t} + \frac{2\kappa}{\kappa^2 + \chi^2}\big[\kappa e^{\kappa t}(C_2 \cos(\chi t) \pm C_3 \sin(\chi t)) \\ \mp \chi e^{\kappa t}(C_3 \cos(\chi t) \mp C_2 \sin(\chi t))\big]\big]\Big\}. \end{aligned} \tag{S22}$$

The general solution of the original equation is recovered by making the integration constant $C_4$ a function of the other integration constants : $C_4 = f(K_1, K_2, K_3, K_4)$, that is $C_4 = f(e^{-\frac{\kappa t}{2}}(\cos(\frac{\chi t}{2})x_1 \mp \sin(\frac{\chi t}{2})y_1), e^{-\frac{\kappa t}{2}}(\pm\sin(\frac{\chi t}{2})x_1 + \cos(\frac{\chi t}{2})y_1), e^{-\frac{\kappa t}{2}}(\cos(\frac{\chi t}{2})x_2 \mp \sin(\frac{\chi t}{2})y_2), e^{-\frac{\kappa t}{2}}(\sin(\pm\frac{\chi t}{2})x_2 + \cos(\frac{\chi t}{2})y_2))$.

To evaluate the unknown function $f$, we use the initial condition $\Phi_0$ at $t = 0$:

$$\Phi_0(x_1 + iy_1, x_2 + iy_2) = f(x_1, y_1, x_2, y_2)\exp\{-\frac{1}{2}\big[C_1 + \frac{2\kappa}{\kappa^2 + \chi^2}\big[\kappa C_2 \mp \chi C_3\big]\}. \tag{S23}$$

Therefore $C_4$ is given by

$$C_4 = \Phi_0(e^{-\frac{\kappa t}{2} \mp i\frac{\chi t}{2}}\xi, e^{-\frac{\kappa t}{2} \pm i\frac{\chi t}{2}}\eta)\exp\{\frac{1}{2}\big[C_1 + \frac{2\kappa}{\kappa^2 + \chi^2}\big[\kappa C_2 \mp \chi C_3\big]\}. \tag{S24}$$

The last step to get a general expression for the solution is to express the constants $C_1, C_2, C_3$ in the original variables $\xi$ and $\eta$:

$$\begin{aligned} C_1 &= (|\xi|^2 + |\eta|^2)e^{-\kappa t}, \\ C_2 &= \frac{1}{2}(\xi\eta e^{\pm i\chi t} + \xi^*\eta^* e^{\mp i\chi t})e^{-\kappa t}\sinh(2\mathrm{r}), \\ C_3 &= (\frac{i}{2}\cos(\chi t)(\xi\eta^* - \xi^*\eta) \pm \frac{1}{2}\sin(\chi t)(\xi\eta + \xi^*\eta^*))e^{-\kappa t}. \end{aligned} \tag{S25}$$

Plugging this into the expression of $C_4$ and $\Phi$, we finally obtain the general expression for the characteristic function :

$$\Phi(t,\xi,\eta) = \Phi_0(e^{-\frac{\kappa t}{2}\mp i\frac{\chi t}{2}}\xi, e^{-\frac{\kappa t}{2}\pm i\frac{\chi t}{2}}\eta)\exp\{\frac{1}{2}e^{-\kappa t}g(t,\xi,\eta)\}$$
$$\times\ \exp\{-\frac{1}{2}[(|\xi|^2+|\eta|^2)\cosh(2\mathrm{r}) + (\kappa(\xi\eta+\xi^*\eta^*)\pm i\chi(\xi\eta-\xi^*\eta^*))\frac{\kappa}{\kappa^2+\chi^2}\sinh(2\mathrm{r})]\}, \quad \text{(S26)}$$

where

$$g(t,\xi,\eta) = |\xi|^2+|\eta|^2+\frac{\kappa}{\kappa^2+\chi^2}\big[\kappa(\xi\eta e^{\pm i\chi t}+\xi^*\eta^* e^{\mp i\chi t})\sinh(2\mathrm{r})$$
$$\mp\chi\cos(\chi t)(\xi\eta^*-\xi^*\eta) - \chi\sin(\chi t)(\xi\eta+\xi^*\eta^*)\big]. \quad \text{(S27)}$$

Noting that $\Phi_0(0,0)=1$ and that $g(t,\xi,\eta)$ is a bounded function of time, $\Phi(t,\xi,\eta)$ converges exponentially at rate $\kappa$ to $\Phi_f(\xi,\eta)$, where $\Phi_f(\xi,\eta)$ is given by

$$\Phi_f(\xi,\eta) = \exp\{-\frac{1}{2}[(|\xi|^2+|\eta|^2)\cosh(2\mathrm{r}) + (\kappa(\xi\eta+\xi^*\eta^*)\pm i\chi(\xi\eta-\xi^*\eta^*))\frac{\kappa}{\kappa^2+\chi^2}\sinh(2\mathrm{r})]\}$$
$$= \exp\{-\frac{1}{2}[(|\xi|^2+|\eta|^2)\cosh(2\mathrm{r}) + \alpha\xi\eta+\alpha^*\xi^*\eta^*]\}. \quad \text{(S28)}$$

with $\alpha = \alpha_r + i\alpha_i = \cos(\theta)\sinh(2r)e^{i\theta}$, $\theta$ being defined by $\tan(\theta) = \pm\frac{\chi}{\kappa}$.

To characterize the gaussian steady state $\Phi_f$, it is useful to rewrite it using the standard form of a characteristic function of a gaussian state

$$\Phi_f(\xi,\eta) = \exp\{-\frac{1}{2}(\xi,\eta)R\sigma R^T(\xi,\eta)^T\}, \quad \text{(S29)}$$

where $(\xi,\eta) = (\mathrm{Re}(\xi),\mathrm{Im}(\xi),\mathrm{Re}(\eta),\mathrm{Im}(\eta))$, $R$ is the symplectic matrix $R=\widetilde{R}\oplus\widetilde{R}$; $\widetilde{R}=\begin{pmatrix}0 & 1\\ -1 & 0\end{pmatrix}$, and the covariance matrix $\sigma$ is given by

$$\sigma = \begin{pmatrix} \cosh(2\mathrm{r})\mathcal{I}_2 & \begin{matrix}-\alpha_r & \alpha_i\\ \alpha_i & \alpha_r\end{matrix} \\ \begin{matrix}-\alpha_r & \alpha_i\\ \alpha_i & \alpha_r\end{matrix} & \cosh(2\mathrm{r})\mathcal{I}_2\end{pmatrix}.$$

This gaussian state is a two mode squeezed thermal state, characterized by the squeezing parameter $\xi' = r'e^{i\theta}$, where $\theta$ is defined by $\tan(\theta) = \pm\frac{\chi}{\kappa}$ and the squeezing strength $r'$ is defined by $\tanh(2r') = \cos(\theta)\tanh(2r)$, and by the mean number of thermal photons $n_{th} = \frac{1}{2}(\sqrt{1+\sin^2(\theta)\sinh^2(2r)}-1)$.

## 2. *Maximum rate of convergence analysis*

As explained in the main text, for a fixed Rabi rate, the highest rate of convergence is achieved for a finite value of the squeezing strength. This behavior is the result of the following competing phenomena. First, the stabilization process is activated by the fluctuations of the population imbalance $\hat{M}$ by the two-mode squeezed thermal state. More precisely, $\sqrt{\langle\hat{M}^2\rangle} = \frac{1}{\sqrt{2}}|\sin(\theta)|\sinh(2r)$ that increases with amplification strength. Second, the pointer state of the cavities is a two-mode squeezed vacuum state in the odd qubit subspace and a two-mode squeezed thermal state in the even qubit subspace. The coupling between the two subspaces is performed by the qubit drive and for small drive strength, $\Omega \ll \kappa,\chi$, the oscillation rate is given by $\Omega\mathrm{tr}\{\hat{\rho}_{\mathrm{SV}}\hat{\rho}_{\mathrm{ST}}\}$ that decreases with amplification strength.

## II. THREE-WAVE MIXER IN THE CONVERSION MODE

We derive the effective single mode model from the description of the whole system including harmonics in the long resonators. To proceed, we build the vector $\mathbf{a}$ of the bare modes sorted as follows: $\hat{a}_1$, $\hat{a}_2$, $\hat{c}_1$, $\hat{c}_2$, $\hat{f}_{1n}$, $\hat{f}_{2n}$ ($\mathcal{N}$ modes in total). The Hamiltonian without qubits and drives is then diagonalized, $\hat{H}_0 = \sum_n E_n \hat{A}_n^\dagger \hat{A}_n$, where the vector of eigenmodes $\mathbf{A}$ is sorted such that $\hat{d}_1$ and $\hat{d}_2$ are the first eigenmodes. We define the matrix $\mathbf{P}$ with the relation $\mathbf{a} = \mathbf{PA}$. We go to the frame rotating at $E_1$ for all eigenmodes, where $\hat{H}_0 = \sum_{n>1} \Delta E_n \hat{A}_n^\dagger \hat{A}_n$ with $\Delta E_n = E_n - E_1$. The dispersive couplings and the cavity drives will give a coupling between the eigenmodes and drive them.

The coupling to qubits reads

$$\hat{H}_{rq} = -\tfrac{1}{2}\chi_1 \hat{\sigma}_{z1} \hat{a}_1^\dagger \hat{a}_1 - \tfrac{1}{2}\chi_2 \hat{\sigma}_{z2} \hat{a}_2^\dagger \hat{a}_2 \tag{S30}$$

$$= -\sum_{n,m=1}^{\mathcal{N}} \tfrac{1}{2}\left[\chi_1 \mathbf{P}_{1n}\mathbf{P}_{1m}\hat{\sigma}_{z1} + \chi_2 \mathbf{P}_{2n}\mathbf{P}_{2m}\hat{\sigma}_{z2}\right] \hat{A}_n^\dagger \hat{A}_m. \tag{S31}$$

The dispersive couplings to eigenmode $\hat{A}_1$ are tuned with $\Delta$ to get equal dispersive shifts $\chi$ to each qubits, $\tilde{\chi}_{11} = \tilde{\chi}_{21} \equiv \chi$, where we note $\tilde{\chi}_{jn} = \chi_j \mathbf{P}_{jn}^2$. Note that here we use a tilda instead of the subscript "eff" for a lighter notation.

$$\hat{H}_{rq} = -\tfrac{1}{2}\chi(\hat{\sigma}_{z1} + \hat{\sigma}_{z2})\hat{A}_1^\dagger \hat{A}_1 - \sum_{\substack{n,m=1\\(n,m)\neq(1,1)}}^{\mathcal{N}} \tfrac{1}{2}\left[\chi_1 \mathbf{P}_{1n}\mathbf{P}_{1m}\hat{\sigma}_{z1} + \chi_2 \mathbf{P}_{2n}\mathbf{P}_{2m}\hat{\sigma}_{z2}\right] \hat{A}_n^\dagger \hat{A}_m. \tag{S32}$$

Two drives are then applied on cavity 1, at frequencies $\omega_{\mathrm{d}a1,1} = \omega_{a1} + \Delta + E_1 + \chi$ and $\omega_{\mathrm{d}a1,2} = \omega_{a1} + \Delta + E_1 - \chi$ to drive eigenmode $A_1$ when qubits are in states $|gg\rangle$ or $|ee\rangle$. The driving Hamiltonian reads

$$\hat{H}_{\mathrm{dr}} = 2\cos(\chi t) \sum_{n=1}^{\mathcal{N}} \tilde{\epsilon}_n \left[\hat{A}_n^\dagger + \hat{A}_n\right], \tag{S33}$$

with $\tilde{\epsilon}_n = \mathbf{P}_{1n}\epsilon$. The bare Lindbladian consists of a dissipator for each mode. In terms of the eigenmodes, this induces a dissipative coupling between all modes. The total Lindbladian reads

$$L = \sum_n \tilde{\kappa}_n D[A_n] + \sum_{n<m} \tilde{\kappa}_{nm} C[A_n, A_m], \tag{S34}$$

with $C[\hat{A}_1, \hat{A}_2]\cdot = \hat{A}_1 \cdot \hat{A}_2^\dagger + \hat{A}_2 \cdot \hat{A}_1^\dagger - \frac{1}{2}\{\hat{A}_1^\dagger \hat{A}_2 + \hat{A}_2^\dagger \hat{A}_1, \cdot\}$,

$$\tilde{\kappa}_n = \sum_k \kappa_k \mathbf{P}_{kn}^2, \qquad \tilde{\kappa}_{nm} = \sum_k \kappa_k \mathbf{P}_{kn}\mathbf{P}_{km}, \tag{S35}$$

where $\vec{\kappa}$ is the vector of damping rates of $\mathbf{a}$. If the damping rate is the same for all modes, $\tilde{\kappa}_n = \kappa$.

The Hamiltonian is QND for the qubits, so the qubits state remains constant. We set the qubits state to $|j_1, j_2\rangle$ and compute the dynamics of the average value of the eigenmodes, $\langle \hat{A}_n^{j_1 j_2}\rangle$. The system being quadratic, this is a closed system. The equations of motion read

$$\partial_t \langle \hat{A}_n \rangle = -2i\tilde{\epsilon}_n \cos(\chi t) - \left[i(\Delta E_n - \tfrac{1}{2}\chi_{nn}^{j_1 j_2}) + \tfrac{1}{2}\tilde{\kappa}_n\right]\langle \hat{A}_n \rangle + \sum_{m\neq n}\left[i\tfrac{1}{2}\chi_{nm}^{j_1 j_2} - \tfrac{1}{2}\tilde{\kappa}_{nm}\right]\langle \hat{A}_m \rangle, \tag{S36}$$

with

$$\chi_{nm}^{j_1 j_2} = \chi_1 \mathbf{P}_{1n}\mathbf{P}_{1m}\langle j_1|\hat{\sigma}_{z1}|j_1\rangle + \chi_2 \mathbf{P}_{2n}\mathbf{P}_{2m}\langle j_2|\hat{\sigma}_{z2}|j_2\rangle. \tag{S37}$$

The drive strength is set by $(2\tilde{\epsilon}_1/\tilde{\kappa}_1)^2 = \bar{n}$ to displace the $\hat{A}_1$ mode by $\sqrt{\bar{n}}$ in the steady state. The set of linear differential equations Eq. (S36) can be expressed with matrices, $\partial_t \langle \mathbf{A} \rangle = -2i\vec{\epsilon}\cos(\chi t) - i\mathbf{VA}$, and diagonalized, $\mathbf{V} = \mathbf{PDP}^{-1}$ with $\mathrm{Im}\{\mathbf{D}_n\} \geq 0$. The equations are integrated into

$$\mathbf{A}(t) = -2i\mathbf{P}\int_0^t \mathrm{d}t' \mathrm{e}^{-i\mathbf{D}(t-t')}\cos(\chi t')\mathbf{P}^{-1}\vec{\epsilon}$$

$$= \mathbf{P}\left\{\frac{\mathrm{e}^{-i\mathbf{D}t} - \mathrm{e}^{-i\chi t}}{\mathbf{D} - \chi} + \frac{\mathrm{e}^{-i\mathbf{D}t} - \mathrm{e}^{i\chi t}}{\mathbf{D} + \chi}\right\}\mathbf{P}^{-1}\vec{\epsilon}. \tag{S38}$$

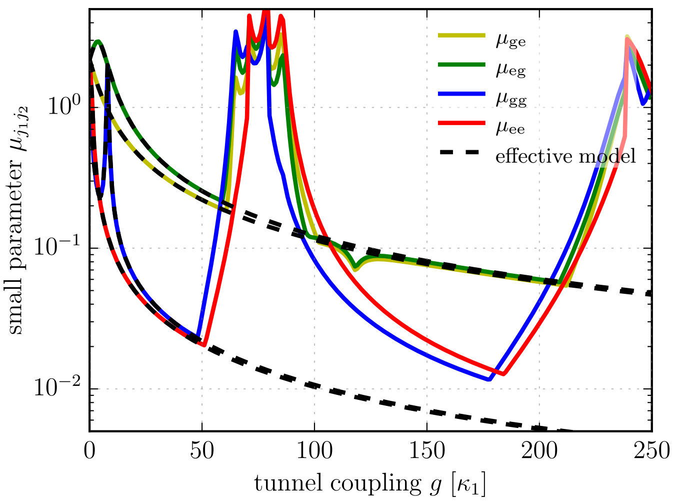


FIG. S1. Parameter $\mu_{j_1j_2}$ for the 4 two-qubit states, obtained for $\bar{n} = 4$. The mostly unwanted driven eigenmode is $\hat{A}_2$.

To attest that the physics is effectively single mode, we show that the modes $\hat{A}_{n>1}$ are not displaced. We define the parameter $\mu$ as

$$\frac{\max_{n>1}\left\{\max_t\left\{|\langle\hat{A}_n^{j_1j_2}\rangle(t)|\right\}\right\}}{|\langle\hat{A}_1^{j_1j_2}\rangle(t\to\infty)|} \leq \mu_{j_1j_2} = \frac{\max_{n>1}\left\{2\sqrt{|(\mathbf{V}-\chi)^{-1}\vec{\epsilon}|_n^2+|(\mathbf{V}+\chi)^{-1}\vec{\epsilon}|_n^2}\right\}}{\sqrt{|(\mathbf{V}-\chi)^{-1}\vec{\epsilon}|_1^2+|(\mathbf{V}+\chi)^{-1}\vec{\epsilon}|_1^2}}, \tag{S39}$$

that is small when the dynamics involves only the eigenmode $\hat{A}_1$.

The dependence of the couplings $\tilde{g}_n$ on the harmonic index $n$ is $\tilde{g}_n = \sqrt{n+1}\tilde{g}_0$ [S4]. We keep the damping rates constant $\kappa_n = \kappa$. We use the parameters of the experiment Ref. S4 for the long resonator $\hat{f}_1$:

$$L_{f1} = 68\,\text{cm}, \qquad \omega_{f1} = 92\,\text{MHz}, \qquad n_0 = 75, \qquad \kappa_{f1,75} = 1\,\text{MHz}, \qquad \tilde{g}_{a1,75} = \tilde{g}_{c1,75} = 500\,\text{MHz}, \tag{S40}$$

for $\kappa_1 = \kappa_2 = 1\,\text{MHz}$ and $\omega_{a1} = \omega_{a2} = 6.9\,\text{GHz}$. For the long resonator $\hat{f}_2$, we take it 1.2 times longer,

$$L_{f2} = 81.6\,\text{cm}, \qquad \omega_{f2} = 76.7\,\text{MHz}, \qquad m_0 = 90, \qquad \kappa_{f2,90} = 1\,\text{MHz}, \qquad \tilde{g}_{a2,90} = \tilde{g}_{c2,90} = 500\,\text{MHz}. \tag{S41}$$

The results are plotted in Fig. S1. The $\chi$ mismatch is corrected at $G = 168\,\text{MHz}$ where $E_1 \simeq 21\chi$, $\mu_{gg,ee} \simeq 0.01$, $\mu_{ge,eg} \simeq 0.07$. The mostly unwanted driven eigenmode is $A_2$. This parasitic driving can be suppressed by driving cavity 2 with the appropriate strengths. With this we get $\mu_{gg,ee} \simeq 0.004$, $\mu_{ge,eg} \simeq 0.05$.

## Effective model

Out of specific resonances, the most driven eigenmode after the mode of interest $A_1$ is the eigenmode $A_2$. We can study the full quantum dynamics of the modes $A_1$ and $A_2$ coupled to the two qubits with the effective Hamiltonian,

$$\begin{aligned}\hat{H}_{\text{eff}} = &-\tfrac{1}{2}\chi(\hat{\sigma}_{z1}+\hat{\sigma}_{z2})\hat{A}_1^\dagger\hat{A}_1 + 2\tilde{\epsilon}_1\cos(\chi t)[\hat{A}_1^\dagger+\hat{A}_1] + \Omega[\hat{\sigma}_{x1}+\hat{\sigma}_{x2}+(\hat{\sigma}_{1-}-\hat{\sigma}_{2-})\mathrm{e}^{-i\bar{n}\chi t}+(\hat{\sigma}_{1+}-\hat{\sigma}_{2+})\mathrm{e}^{i\bar{n}\chi t}]\\ &-(E_1-E_2)\hat{A}_2^\dagger\hat{A}_2 - \tfrac{1}{2}(\tilde{\chi}_{12}\hat{\sigma}_{z1}+\tilde{\chi}_{22}\hat{\sigma}_{z2})\hat{A}_2^\dagger\hat{A}_2 + 2\tilde{\epsilon}_2\cos(\chi t)[\hat{A}_2^\dagger+\hat{A}_2] - \tfrac{1}{2}[\mathcal{X}_1\hat{\sigma}_{z1}+\mathcal{X}_2\hat{\sigma}_{z2}][\hat{A}_1^\dagger\hat{A}_2+\hat{A}_2^\dagger\hat{A}_1]\\ &-\tfrac{1}{2}\Lambda\hat{\sigma}_{z1}\hat{\sigma}_{z2},\end{aligned} \tag{S42}$$

with $\mathcal{X}_j = \chi_j\mathbf{P}_{j1}\mathbf{P}_{j2}$. The first line of the effective Hamiltonian represents the single mode Hamiltonian required to stabilize Bell states, the second line describes the coupling to the second mode. The last line is the $\hat{\sigma}_z\hat{\sigma}_z$ coupling induced by the other eigenmodes, obtained from the factorization $\sum_j \chi_j\hat{\sigma}_{zj}\sum_{n,m=3}^{\mathcal{N}}\mathbf{P}_{jn}\mathbf{P}_{jm}\hat{A}_n^\dagger\hat{A}_m \approx$

$\sum_j \chi_j \hat{\sigma}_{zj} \sum_{n,m=3}^{\mathcal{N}} \mathbf{P}_{jn}\mathbf{P}_{jm}\langle \hat{A}_n^\dagger \hat{A}_m\rangle$, with the strength

$$\Lambda = \lambda_1^{11} + \lambda_2^{11} - \lambda_1^{00} - \lambda_2^{00} + \lambda_1^{01} - \lambda_2^{01} - \lambda_1^{10} + \lambda_2^{10}, \tag{S43}$$

$$\lambda_j^{j_1 j_2} = \tfrac{1}{4}\chi_j \sum_{n,m=3}^{\mathcal{N}} \mathbf{P}_{jn}\mathbf{P}_{jm}\langle \hat{A}_n^\dagger \hat{A}_m\rangle_{j_1 j_2}. \tag{S44}$$

These terms also renormalize the qubit frequency, $\delta\omega_{q1} = \lambda_1^{11} + \lambda_2^{11} + \lambda_1^{00} + \lambda_2^{00} + \lambda_1^{01} + \lambda_2^{01} + \lambda_1^{10} + \lambda_2^{10}$ and $\delta\omega_{q2} = \lambda_1^{11} + \lambda_2^{11} + \lambda_1^{00} + \lambda_2^{00} - \lambda_1^{01} + \lambda_2^{01} - \lambda_1^{10} + \lambda_2^{10}$. There are in practice tiny and neglected.
The Lindbladian reads $L_{\mathrm{eff}} = \tilde{\kappa}_1\mathcal{D}[\hat{A}_1] + \tilde{\kappa}_2\mathcal{D}[\hat{A}_2] + \tilde{\kappa}_{12}\mathcal{C}[\hat{A}_1, \hat{A}_2]$.
In practice, $\Delta$ is determined to correct the dispersive shifts asymmetry, the drive strength is set to $\epsilon_1 = \frac{\tilde{\kappa}_1\sqrt{\bar{n}}}{2\mathbf{P}_{11}}$ and the qubit drive amplitude is set to $\Omega = \frac{1}{2}\tilde{\kappa}_1$.

When one harmonic is considered in each long resonator and this harmonic is at resonance with both cavity and TWM modes, the energy separation is equal to $E_1 - E_2 = \hbar g \dfrac{\chi_1 + \chi_2}{\sqrt{\chi_1\chi_2}} \sin^2\varphi$ and the dispersive shift is equal to $\chi = \dfrac{\chi_1\chi_2}{\chi_1 + \chi_2}\cos^2\varphi$.


[S1] C. Le Bris and P. Rouchon, Phys. Rev. A **87**, 022125 (2013).
[S2] S. M. Barnett and P. M. Radmore, *Methods in Theoretical Quantum Optics* (Oxford University Press, 2003).
[S3] S. Haroche and J. Raimond, *Exploring the Quantum: Atoms, Cavities and Photons.* (Oxford University Press, 2006).
[S4] N. M. Sundaresan, Y. Liu, D. Sadri, L. J. Szőcs, D. L. Underwood, M. Malekakhlagh, H. E. Türeci, and A. A. Houck, Phys. Rev. X **5**, 021035 (2015).
